# Supplementary material for: The Complexity of Verifying Population Protocols
Source: arXiv:1912.06578 source file (2021-02-09)
Supplement: Supplementary file 1 [file appendix-observation-section.tex]

\section{Appendix for Section \ref{sec:io-hardness}}%%%%%%%%%%%%%%%%%%%

The following definition and lemma are introduced to help  prove that our IO protocol implementation of a Turing machine does indeed simulate its functioning.
To recall the notation, let us start with an illustration of transitions modelling a single step of the Turing machine into the protocol.
The fragment of the protocol is represented as a Petri net whose places and transitions represent the states and transitions of the IO protocol.

\input figure-turing-io.tex

Figure~\ref{figure-turing-io} illustrates transitions involved in modelling a single step of a Turing machine
that reads $0$, writes $1$, moves head to the right and switches the control state from $q$ to $q'$.

\begin{definition}
 A configuration of $\PP_M$ is a \emph{modelling configuration} if the following conditions hold.
\begin{enumerate}
        \item For every $1\leq n\leq K$ exactly one of the $2|\Sigma|$ states 
        $\act{\sigma}{n}, \pass{\sigma}{n}$ is populated, and it is populated with a single agent. \\
        (Intuitively: every cell is either \textit{on} or \textit{off} and contains exactly one symbol.)
        \item Exactly one of all the head states is populated (again, with a single agent).
        \item If a cell state $\act{\sigma}{n}$ is populated, then a head state $\stable{q}{n}$ or $\switch{q}{\sigma'}{n}{d}$ is populated for some $\sigma'$ and $d$.
        \item If a head state $\switch{q}{\sigma}{n}{d}$ is populated,
                either $\act{\sigma'}{n}$ is populated for some $\sigma'$,
                of $\pass{\sigma}{n}$ is populated.
\end{enumerate}
\end{definition}

\begin{remark}
Note that for every configuration $c$ of $M$ the configuration $C_c$ described in Definition \ref{def:turing-configuration} is a modelling configuration.
\end{remark}

\begin{lemma}
        \label{lemma:modellingmarkingevolution}
For every modelling configuration $C$ of $\PP_M$:
\begin{itemize}
\item[(1)] $C$ enables at most one transition.
\item[(2)] If $C$ enables no transitions, then it populates states $\act{\sigma}{n}$ and $\stable{q}{n}$ for some $q \in Q$, $\sigma \in \Sigma$, and $1 \leq n \leq K$.
\item[(3)] If $C \trans{} C'$, then $C'$ is also a modelling configuration. 
\end{itemize}
\end{lemma}
\begin{proof}
\noindent (1) All possible transitions require agents at two states,
        one of type $\act{\cdot}{n}$ or $\pass{\cdot}{n}$
        and one of type $\stable{\cdot}{n}$ or $\switch{\cdot}{n}{\cdot}{\cdot}$, with the same $n$.
        But the modelling condition requires that there can be at most one such pair.

\noindent (2) If a $\switch{\cdot}{\cdot}{\cdot}{\cdot}$ state is populated,
        a transition is always possible by definition
        of the list of $\switch{\cdot}{\cdot}{\cdot}{\cdot}$ states.
        The same for the case where a $\stable{\cdot}{\cdot}$ state
        is populated but no $\act{\cdot}{\cdot}$ case is populated.
        If there are populated states of types $\act{\cdot}{n}$ and $\stable{\cdot}{n}$,
        the transition may fail
        to exist if either the Turing machine halts or if it goes outside the allocated space.

\noindent (3) Every transition consumes and produces one agent 
        at $\pass{\cdot}{n}$ or $\act{\cdot}{n}$ state,
        and the new state has the same $n$.
        Every transition consumes and produces one agent
        at $\switch{\cdot}{\cdot}{\cdot}{\cdot}$ or $\stable{\cdot}{\cdot}$ state.
        If an $\act{\cdot}{n}$ state becomes populated after a transition,
        it has the same $n$ as the populated $\stable{\cdot}{n}$ state
        of both configurations (before and after);
        if an $\act{\cdot}{n}$ state stays populated,
        the agent is moved from a $\stable{\cdot}{n}$ to a $\switch{\cdot}{n}{\cdot}{\cdot}$
        state with the same $n$.
When $\switch{q}{\sigma}{n}{d}$ becomes populated,
        the transition needs a populated $\act{\cdot}{n}$ state.
        When $\switch{q}{\sigma}{n}{d}$ stays populated,
        the transition populates a $\pass{\sigma}{n}$ state.
        
 \end{proof}

\theoremSimulationStep*
\begin{proof}
        By Lemma~\ref{lemma:modellingmarkingevolution},
        for all $c$ there is either zero or one possibility for the
sequence $t_1,t_2,t_3,t_4$ starting in $C_c$. 
        It is easy to see from the definition of steps configuration $\switch{\cdot}{\cdot}{\cdot}{\cdot}$
        states that if such a sequence exists, it results in $c'$ such that $c\trans{}c'$.
        If such a sequence doesn't exist, the failure must occur when trying to populate
        a  $\switch{\cdot}{\cdot}{\cdot}{\cdot}$ state. 
        In that case the configuration~$c$ must be blocked, either by
        the transition being undefined or by going out of bounds.
 \end{proof}

\ThmIOCorrectnessHard*
\begin{proof}
Let $p$ be a fixed polynomial satisfying $p(n) \geq n$ for all $n$. 
Consider the set of deterministic Turing machines whose set of states contains two distinct distinguished states $q_{acc}, q_{rej}$,  and whose computation on empty tape satisfies the following conditions:
\begin{itemize}
\item The computation never visits a configuration that visits more than $p(n)$ cells, where $n$ is the size of the Turing machine $M$,
and visits the set $\{q_{acc}, q_{rej}\}$ of states exactly once.
\item The computation ends in a configuration $c$ with empty tape and control state either $q_{acc}$ or $q_{rej}$. 
\end{itemize}
We say that the machine \emph{accepts} (\emph{rejects}) if it terminates in $q_{acc}$ ($q_{rej}$). 
It is well known that the problem whether such a machine accepts on empty tape is \PSPACE-hard. 
Because co\PSPACE=\PSPACE, the complement of this problem is also in \PSPACE and this is what we reduce to a correctness problem for a specific IO protocol and predicate.

Given such a machine $M$ with initial state $q_{init}$ and a size bound, let $\PP_M$ be its IO protocol implementation, defined in Section \ref{sec:io-hardness}.
%Let $C_0$ and $C$ be the modeling configurations describing the initial configuration and the unique accepting configuration.  Then $M$ accepts if{}f $C$ is reachable from $C_0$ if{}f some configuration reachable from $C_0$ covers the configuration that puts a agent in the state for $q_{acc}$.
We add two additional states to $\PP_M$, $observer$
        and $success$. We add the following transitions: 
        \begin{itemize}
	\item$(\stable{q_{acc}}{\cdot},observer) \mapsto (\stable{q_{acc}}{\cdot},success$), and
	\item$(success, \cdot) \mapsto (success, success)$.
	\end{itemize}
We also add transitions such that if there are two agents in the head states,
        or two agents in the cell states for the same cell,
        or two agents in the $observer$ state,
        one of them can move to $success$.
       
        The input states are $\pass{0}{\cdot}$, $\stable{q_{init}}{1}$ and the $observer$ state.
        The output function is $1$ for $success$ and $0$ otherwise.
        We define a predicate as ``there are at least two agents in the head states,
        or at least two agents in the cell states for some cell, or at least two agents in the $observer$ state''.

        If the Turing machine accepts the empty tape without going out of bounds,
        the protocol is not correct, as we can put exactly one agent in every 
        input and run the simulation until the acceptance will lead to one of the
        $(\stable{q_{acc}}{\cdot},observer) \mapsto (\stable{q_{acc}}{\cdot},success)$ transitions firing.

        Otherwise the protocol is correct, as there are configurations not greater than the
        configuration with one agent in every input state, which cannot populate the $success$ 
        state because the bounding configuration cannot;
        the remaining configurations are accepted by the predicate and will also converge
        to all the agents being in the $success$ state.
        
        So this construction reduces non-acceptance on an empty tape of a Turing machine of bounded tape to correctness of this protocol.
        This construction also reduces non-acceptance on an empty tape of a Turing machine of bounded tape to single-instance correctness of this protocol over the initial configuration that puts exactly one agent in every input state.
 \end{proof}

\section{Appendix for Section \ref{sec:pruning}}%%%%%%%%%%%%%%%%%%%

\LemmaRealizableMFDO*
\begin{proof}
One direction is obvious by definition: if we have a realizable extended history (even not well-structured),
it also describes a run.
Let us prove the other direction.

Informally, we just implement the de-anonymisation of the agents.
A formal proof can be given by induction in the number of transitions in the run.

\noindent
\emph{Base case}. If there are no transitions, we create a multiset of trajectories of length one such that the initial states of the trajectories are exactly the states (with multiplicity) of the initial configuration of the run.
This is well-structured because there are no steps.
We define the initial seen set of the history to be the initial seen set of the configuration (which therefore satisfies the requirement of containing at least the populated states of the configuration).

\noindent
\emph{Induction step}. Consider a sequence of transitions and a corresponding well-structured extended history.
Now let us add a single enabled transition. 
To build the new extended history, we choose an arbitrary trajectory of the existing history such that this trajectory ends in the state corresponding to the source state of the added transition.
Such a trajectory exists because the transition is enabled and therefore its source state must be populated.
We extend the chosen trajectory with a step from the source state to the destination state of the added transition,
and we extend the rest of the trajectories with one horizontal step each.
If the seen set of the previous final configuration did not contain the destination state, we add it to the new final seen set.
We obtain a multiset of trajectories of same length, thus constituting a history.
It is realizable using the considered sequence of transitions followed by the new enabled transition.
As we add only a single non-horizontal step at that moment of time, we cannot
break the well-structuring condition.
 \end{proof}

\LemmaHistoryMFDO*
\begin{proof} 
Let a well-structured extended history $(H,\seen_H)$ be realizable in $\PP$.
Consider an arbitrary non-horizontal step $\tau(i) \tau(i+1)=q q'$ in some trajectory of this history.
All the non-horizontal steps at the corresponding position in $H$ are equal by well-structuredness,
and realizability implies that there is a transition of $\PP$
with source state $q$ and destination state $q'$ enabled at extended configuration $(C_H^i,\seen_H^i)$.
%This transition can be applied as many times as there are equal steps 
%at the corresponding position in $H$.
Therefore the observed state $o$ of this transition is in $\seen_H^i$.
As this holds for each non-horizontal step in $H$, $(H,\seen_H)$ is compatible with $\PP$.

Now assume that $(H,\seen_H)$ is compatible with $\PP$.
If some position in $H$ contains only horizontal steps,
we can use the empty transition $t_{\varepsilon}$.
If a position contains some number of (equal by well-structuredness) non-horizontal steps
$q q'$, its seen set also contains a state $o$
such that $q \trans{o} q'$ is a transition in $\PP$.
All the other steps at the corresponding position are horizontal.
Therefore we can iterate the transition $q \trans{o} q'$ by the number of non-horizontal steps
to obtain the next configuration.
 \end{proof}

\LemmaRealizableIO*
\begin{proof}
The proof is the same as for MFDO, except that we ignore the part about seen sets.
 \end{proof}

\LemmaHistoryIO*
\begin{proof} 
Let a well-structured history $H$ be realizable in $\PP$.
Consider an arbitrary non-horizontal step $\tau(i) \tau(i+1)=q q'$ in some trajectory of this history.
All the non-horizontal steps at the corresponding position in $H$ are equal by well-structuredness,
and realizability implies that there is a transition of $\PP$
with source state $q$ and destination state $q'$ enabled at configuration $C_H^i$.
This transition can be applied as many times as there are equal steps 
at the corresponding position in $H$.
Therefore the observed state $o$ of this transition is populated both before and after iterating this transition, which corresponds to  $H$ containing a trajectory with the step $o o$ at the corresponding position.
As this holds for each non-horizontal step in $H$, $H$ is compatible with $\PP$.

Now assume that $H$ is compatible with $\PP$.
If some position in $H$ contains only horizontal steps,
we can use the empty transition $t_{\varepsilon}$.
If a position contains some number of (equal by well-structuredness) non-horizontal steps
$q q'$, it also contains a horizontal step $o o$
such that $q \trans{o} q'$ is a transition in $\PP$.
All the other steps at the corresponding position are horizontal.
Therefore we can iterate the transition $q \trans{o} q'$ by the number of non-horizontal steps
to obtain the next configuration.
 \end{proof}

\section{Appendix for Section \ref{sec:coNP}}%%%%%%%%%%%%%%%%%%%

\ThmCCReachability*
\begin{proof}
Lemma \ref{lm:smallminterm} states that for every extended cube $(\mathcal{C},\seen)$ of a finite decomposition into extended cubes of $\mathcal{D}$, for every extended configuration $(c,\seen_c)$ in $\prestar(\mathcal{C}, \seen)$, there is a ``small" cube $\mathcal{C}_c$ such that $(c,\seen_c)$ is in $(\mathcal{C}_c,\seen_c)$ and $(\mathcal{C}_c,\seen_c)$ is completely in $\prestar(\mathcal{C},\seen)$.
So $\prestar(\Conf, \seen) = \cup_{c \in \prestar(\Conf,\seen)} (\Conf_c,\seen_c)$.
But by the norm restrictions on them, there are only a finite number of such ``small" cubes.

So $\prestar(\Conf,\seen)$ is a finite union of extended cubes.
There exists some finite $k$ such that $\prestar(\mathcal{D}) = \cup_{i=1}^k \prestar(\Conf_i, \seen_i)$. 
Each of these $\prestar(\Conf_i, \seen_i)$ is itself a finite union of extended cubes, so $\prestar(\mathcal{D})$ is a finite union of extended cubes.
Thus by definition, $\prestar(\mathcal{D})$ is an extended counting set.

Let $\Gamma$ be the counting constraint defined as the union of the $(\Conf_i,\seen_i)$.
Let $\Gamma'$ be the counting constraint defined as the union of the $\prestar(\Conf_i, \seen_i)$, themselves unions of ``small" extended cubes.
Then by the bounds in Lemma \ref{lm:smallminterm} and by definition of the norms,
$
\unorm{\Gamma'} \leq \unorm{\Gamma}
$ 
and 
$
\lnorm{\Gamma'} \leq \lnorm{\Gamma} + |Q|.
$

The results also hold for $\poststar(\mathcal{D})$. 
Consider the IO protocol $\PP_r$, the ``reverse" of net $\PP = (Q,\Delta)$. 
Protocol $\PP_r$ is defined as $\PP$ but with transition set $\Delta_r$, where $\Delta_r$ has a transition $(q_1, q_2) \mapsto (q_3, q_4)$ if{}f $\Delta$ has a transition $(q_3, q_4) \mapsto (q_1, q_2)$. 
Notice that $\PP_r$ is still an IO protocol.
Then $\poststar(\mathcal{D})$ in $\PP$ is equal to $\prestar(\mathcal{D})$ in $\PP_r$.
 \end{proof}

\section{Appendix for Section \ref{sec:PSPACE}}%%%%%%%%%%%%%%%%%%%

\LemmaSmallCubeIO*
\begin{proof}
Let $C'$ be a configuration of $\prestar(L,U)$.
There exists a configuration $C \in (L,U)$ such that $C' \longrightarrow C$, and $C \geq L$.
The construction from the Pruning Theorem 
applied to this run
yields configurations $D',D$ such that 
\begin{center}
\(
\begin{array}[b]{@{}c@{}c@{}c@{}c@{}c@{}c@{}c@{}}
C' &  \trans{\hspace{1em}*\hspace{1em}} & C & \  \geq \ &L  \\[0.1cm]
\geq &  & \geq \\[0.1cm]
D' & \trans{\hspace{1em}*\hspace{1em}} &D  & \geq & L
\end{array}
\)
\end{center}
and $|D'| \leq |L| + |Q|^3$.
Since $C$ is in $(L,U)$, we have $U\geq C \geq D \geq L$ and so configuration $D$ is in $(L,U)$ and $D'$ is in $\prestar(L,U)$.

We want to find $L',U'$ satisfying the conditions of the Lemma, i.e. such that $C' \in (L', U')$ and $(L',U') \subseteq  \prestar(L,U)$.
We define $L'$ as equal to configuration $D'$ over each state of $Q$.
The following part of the proof plays out in the setting of the Pruning Theorem section, in which the tokens are de-anonymized. 
Let $H_C$ be a well-structured realizable history from $C'$ to $C$. 
Let $q$ be a state of $Q$.
We want to define $U'(q)$.
Consider $\mathcal{B}^C_q$ the set of bunches in history $H_C$ that have $q$ as an initial state.
For every bunch $B$, let $f_B$ be the final state of the bunch.
We define $U'(q)$ depending on the final states of bunches in $\mathcal{B}^C_q$.

\noindent
\emph{Case 1.} 
There exists a bunch $B$ in $\mathcal{B}^C_q$ whose final state $f_B$ is such that $U(f_B) = \infty$.
In this case we define $U'(q)$ to be $\infty$.

\noindent
\emph{Case 2.}
For all bunches $B$ in $\mathcal{B}^C_q$, the final state $f_B$ of $B$ is such that $U(f_B) < \infty$.
In this case we define $U'(q)$ to be $\sum_{B \in \mathcal{B}^C_q} size(B)$, where $size(B)$ is the number of trajectories with multiplicity in $B$, and $0$ if $\mathcal{B}^C_q$ is empty.

Let us show that $(L',U')$ has the properties we want.
The number of tokens in configuration $C'$ at state $q \in Q$ is the sum of the sizes of the bunches that start from $q$ in history $H_C$.
That is, $C'(q)=\sum_{B \in \mathcal{B}^C_q} size(B)$ which is exactly $U'(q)$ when $U'(q)$ is finite.
Thus for all $q \in Q$, $C'(q) \leq U'(q)$ and $C'(q) \geq D'(q)=L'(q)$, so $C'$ is in $(L', U')$.

The construction from the Pruning Theorem ``prunes" history $H_C$ from $C'$ to $C$ into a well-structured realizable history $H_D$ from $D'$ to $D$ with the same set of non-empty bunches.
We are going to show that $(L',U') \subseteq \prestar(L,U)$ by ``boosting" the bunches of history $H_D$ to create histories $H_R$ which will start in any configuration $R'$ of $(L',U')$ and end at some configuration $R$ in $(L,U)$.
For any constant $k \in \N$, a bunch $B$ of history $H_D$ is \emph{boosted by k} into a bunch $B'$ by selecting any trajectory $\tau$ in $B$ and augmenting its multiplicity by $k$ to create a new bunch $B'$ of size $size(B) + k$.

\input{figure-boost.tex}

Let $R'$ be a configuration in $(L',U')$.
We construct a new history $H_R$ starting in $R'$, and we prove that its final state is in $(L,U)$.
What we aim to build is illustrated in Figure \ref{figure-boost}.
We initialize $H_R$ as the bunches of history $H_D$.
We call $\mathcal{B}^D_q$ the set of the bunches of $H_D$ starting in $q$.

For $q$ such that there is a bunch $B_D \in \mathcal{B}^D_q$ with infinite $U(f_{B_D})$, i.e. such that $\mathcal{B}^D_q$ is in \emph{Case 1} defined above, we take this bunch $B_D$ and boost it by $R'(q) - D'(q)$ into a new bunch $B_R$. 
Informally, we need not worry about exceeding the bound $U$ on the final state of the trajectories of $B_R$, because this state is $f_{B_D}$ and its upper bound is infinite.
The number of trajectories starting in $q$ in history $H_R$ is now $R'(q)$.

Otherwise, $q$ is such that $\mathcal{B}^D_q$ is in \emph{Case 2}, so we know that $R'(q)\leq C'(q)$ because $U'(q)$ was defined to be $C'(q)$. 
Each bunch in $\mathcal{B}^D_q$ in history $H_D$ has a corresponding bunch in history $H_C$ because the pruning operation never erases a bunch completely, it only diminishes its size.
We can boost all bunches in $\mathcal{B}^D_q$ to the size of the corresponding bunches in $H_C$ and not exceed the finite bounds of $U$ on the final states of these bunches.
We arbitrarily select bunches in $\mathcal{B}^D_q$ which we boost so that the sum of the size of bunches in $\mathcal{B}^D_q$ is equal to $R'(q)$.

Now by construction, history $H_R$ starts in configuration $R'$, and it ends in a configuration $R$ such that $D\leq R\leq U$, as every bunch is either boosted to a size no greater than it had in $H_C$, or leads to a state $q$ with $U(q)=\infty$.
Since $D \geq L$, this implies that $R \geq L$ and so $R \in (L,U)$ and $R' \in \prestar(L,U)$.

Finally, we show that the norms of $(L',U')$ are bounded.
For the $l$-norm, we simply add up the tokens in $D=L'$. 
Thus by the Pruning Theorem
\begin{align*}
\lnorm{(L',U')} \leq |L| + |Q|^3 \leq \lnorm{(L,U)} + |Q|^3.
\end{align*}
By definition of the $u$-norm, 
$\unorm{(L',U')} = \sum_{\substack{q\in Q | U'(q)<\infty}} U'(q).$
If $U'(q)<\infty$ then $\mathcal{B}^C_q$ of history $H_C$ is in Case $2$ and there is no bunch $B\in \mathcal{B}^C_q$ going from $q$ to a final state $f_B$ such that $U(f_B)=\infty$.
So the set of bunches $B$ starting in a state $q$ such that $U'(q)<\infty$ is included in the set of bunches $B'$ such that $U(f_{B'})<\infty$, and thus
\begin{align*}
\sum_{\substack{q\in Q | U'(q)<\infty}} U'(q) = \sum_{\substack{q\in Q | U'(q)<\infty}} \left( \sum_{B \in \mathcal{B}^C_q} size(B) \right)
\leq \sum_{B | U(f_B)<\infty} size(B).
\end{align*}
Now $\sum_{B | U(f_B)<\infty} size(B)$ in history $H_C$ is exactly $\sum_{\substack{q\in Q | U(q)<\infty}} C(q)$.
Since $C \in (L,U)$, for all states we have $C(q)\leq U(q)$ and so 
\begin{align*}
\sum_{\substack{q\in Q | U'(q)<\infty}} U'(q) \leq \sum_{\substack{q\in Q | U(q)<\infty}} C(q)
\leq \sum_{\substack{q\in Q | U(q)<\infty}} U(q).
\end{align*}
So by definition of the norm, $\unorm{(L',U')} \leq \unorm{(L,U)}$.
 \end{proof}

\ThmCCReachabilityIO*
\begin{proof}
The proof is the same as for MFDO, except that we ignore the part about seen sets, and that the norm bound from the Pruning Theorem is cubic in $|Q|$ instead of linear.
 \end{proof}
