# Supplementary material for: The Complexity of Verifying Population Protocols
Source: arXiv:1912.06578 source file (2021-02-09)
Supplement: Supplementary file 2 [file appendix-obs-4-1.tex]

\section{Appendix for Section \ref{sec:mfdo}}%%%%%%%%%%%%%%%%%%

\mr{Fully commented out, what should be here?}
\je{Nothing, can go}
